# Supplementary material for: The Impact of Generative AI Coding Assistants on Developers Who Are Visually Impaired
Source: arXiv:2503.16491 source file (2025-03-10)
Supplement: Supplementary file 1 [file appendix.tex]

\section{Study Questions}
\subsection*{Participant Background \& 
Copilot Experience}
\begin{itemize}
    \item Can you tell us how long you have been working as a professional software developer?
    \item Which programming language do you use most frequently in your projects?
    \item How long have you been using \texttt{<programming language>} as your main programming language?

    \item Have you ever used something like Copilot or ChatGPT for coding?
    \item Can you tell me about a time when you used a tool like Copilot for coding? What worked well and what didn’t?
    \begin{itemize}
        \item Can you share a time when it helped?
        \item Can you share a time when it did not help?
    \end{itemize}
\end{itemize}

\subsection*{Training session}
\begin{itemize}
\item Participants took part in a training session where they were introduced to GitHub Copilot and
its features. The training also covered how Copilot integrates with accessible development environments and assistive
technologies that participants were already using. This session aimed to ensure that all participants started with a
fundamental understanding of how to interact with Copilot during programming tasks.
\end{itemize}

\subsection*{Hands-on coding \& Debugging task}
Each participant was given a moderately complex programming task to
complete using GitHub Copilot in Visual Studio Code, as well as a related debugging task, also to be completed using
GitHub Copilot with Visual Studio Code.
\begin{itemize}

\item \textbf{Programming Task}. Based on prior work [ 33 ], the programming task we selected for participants was to write a
program that takes a string representing the user’s birthday, using their preferred programming language. The string
the user provides is in either the format DDMMYY for day, month, and year, or DDMMYYYY. The program takes the
user’s birthday and should output the number of days until that person’s next birthday. We asked participants to ensure
their solution contains a class that implements all of the date functionality (e.g., it should have a constructor that takes
in the string). We also asked them to write unit tests for the class they created.
Participants were asked to “think aloud,” verbalizing their thought process as they interacted with Copilot and
wrote code. This provided insights into real-time decision-making and interaction patterns. 
\item \textbf{Debugging Task}. Following the initial coding task, a debugging session was conducted where participants needed
to identify and correct any errors in the code generated by Copilot. During this phase, participants were also asked
about various aspects, including their usual approach for evaluating code accuracy, how they dealt with encountered
issues, and their thoughts on whether Copilot made their debugging process simpler or more complex.
\end{itemize}

\subsection*{Post-Study Questions}
\begin{itemize}
    \item I am interested in how you organize code in your head. When you are reading a lot of new code, what is your approach?
    \item When you are writing new code or modifying existing code, how do you plan out what to do in your head or organize your ideas?
    \item How do you usually read through or navigate your code? How did Copilot impact this process?
    \item Does Copilot change how you do this? How?
    \item Did Copilot suggestions change your plan at all?
    \item What was the experience of using Copilot like for you?
    \begin{itemize}
        \item Did it help with completing the task? Why or why not?
        \item What would make Copilot better for you?
        \item What was the most difficult thing about using Copilot?
    \end{itemize}
\end{itemize}

\begin{itemize}
    \item Now that you have used Copilot, what is your feel for the scenarios where you would use it and not use it?
    \item What are your personal concerns regarding using AI in your work?
 %   \item Imagine you are a software developer ten years in the future, and AI technology has advanced significantly. Describe a cutting-edge AI tool or feature that you would like to have to support your programming work. Consider the challenges you face today in software development, such as debugging complex code,
\end{itemize}
